# Supplementary material for: CallNavi, A Challenge and Empirical Study on LLM Function Calling and Routing
Source: arXiv:2501.05255 source file (2025-04-24)
Supplement: Supplementary file 1 [file appendix.tex]

\section{Example Analysis of Hard and Medium Questions}
\label{apd:example}
This section provides an analysis of examples from the \texttt{CallNavi} dataset, focusing on the complexities of medium and hard questions in the bank scenario. The examples illustrate how the tasks test the capabilities of large language models (LLMs) in handling sequential API calls and parameter dependencies.

\subsection{Hard Question Example}
\noindent
\textbf{Question:}  
"I want to travel to Japan, how many Japanese Yen I can spend with my credit card? My customer ID is 123155."  

This question involves reasoning across multiple steps and APIs:
\begin{enumerate}
    \item The model must first retrieve the customer’s credit cards using the \texttt{getCustomerCreditCards} API.
    \item From the retrieved cards, the model must fetch details about a specific credit card using the \texttt{getCreditCardDetails} API.
    \item Finally, the model must compute the currency exchange rate using the \texttt{getCurrencyExchangeRates} API to determine the spending amount in Japanese Yen.
\end{enumerate}
This task tests the model’s ability to maintain dependencies between APIs, as the output of one API (e.g., credit card number) serves as an input for subsequent calls.

\begin{lstlisting}[language=json, caption={Hard Question Example from the Bank Scenario.}, label={lst:hard-question}]
{
  "id": "ban081",
  "question": [
    {
      "role": "user",
      "content": "I want to travel to Japan, how many Japanese Yen I can spend with my credit card? my customer ID is 123155."
    }
  ],
  "ground_truth": {
    "API": ["getCustomerCreditCards", "getCreditCardDetails", "getCurrencyExchangeRates"],
    "parameters": [
      { "customerID": "123155" },
      { "creditCardNumber": "$$$" },
      { "currencyPair": "$$$" }
    ]
  },
  "difficulty": "hard"
}
\end{lstlisting}

\subsection{Medium Question Example}
\noindent
\textbf{Question:}  
"Retrieve details of wire transfer WT987654 and cancel it."  

This question involves two sequential API calls:
\begin{enumerate}
    \item The model must retrieve the details of the wire transfer using the \texttt{getWireTransferDetails} API.
    \item The same transfer ID must then be used to cancel the transaction with the \texttt{cancelWireTransfer} API.
\end{enumerate}
This task evaluates the model’s ability to handle basic sequential tasks with consistent parameter reuse across multiple APIs.

\begin{lstlisting}[language=json, caption={Medium Question Example from the Bank Scenario.}, label={lst:medium-question}]
{
  "id": "ban069",
  "question": [
    {
      "role": "user",
      "content": "Retrieve details of wire transfer WT987654 and cancel it."
    }
  ],
  "ground_truth": {
    "API": ["getWireTransferDetails", "cancelWireTransfer"],
    "parameters": [
      {"transferID": "WT987654"},
      {"transferID": "WT987654"}
    ]
  },
  "difficulty": "medium"
}
\end{lstlisting}

\subsection{Analysis of Model Challenges}
\begin{itemize}
    \item \textbf{Hard Question:} The main challenge lies in maintaining dependencies across APIs and correctly passing intermediate results (e.g., credit card number and currency pair).
    \item \textbf{Medium Question:} While simpler than the hard question, this task requires consistency in parameter reuse (e.g., the same \texttt{transferID} must be used across both API calls).
\end{itemize}
These examples illustrate the varying levels of complexity in the \texttt{CallNavi} dataset, testing the models' abilities to reason through multi-step tasks and maintain logical consistency in API usage.

% \subsubsection*{Key Observations}
% \begin{itemize}
%     \item JSON is more robust for both input and output, offering higher overall performance across tasks.
%     \item YAML introduces significant challenges in both generation and interpretation, particularly in harder tasks.
%     \item Mixed configurations, particularly \textbf{YAML to JSON}, mitigate some YAML-related difficulties, highlighting JSON's simplicity as an output format.
% \end{itemize}

\noindent
These results underscore the importance of selecting appropriate data formats in real-world applications, as structured formats like YAML can introduce unexpected complexities that affect performance. This study also highlights the potential for optimizing LLMs to better handle YAML and similarly complex formats.
